# Supplementary material for: Cooperative Localization for Mobile Networks: A Distributed Belief Propagation - Mean Field Message Passing Algorithm
Source: arXiv:1512.07782 ancillary file (2016-04-03)
Supplement: Supplementary file 1 [file supplementaryMaterial.pdf]

# Cooperative Localization for Mobile Networks: A Distributed Belief Propagation – Mean Field Message Passing Algorithm (Supplementary Material)

Burak Çakmak, Daniel N. Urup, Florian Meyer, Troels Pedersen,
Bernard H. Fleury, and Franz Hlawatsch

April 3, 2016

In this manuscript, we provide a more detailed presentation of the material contained in Section IV-A of the letter "Cooperative Localization for Mobile Networks: A Distributed Belief Propagation – Mean Field Message Passing Algorithm." All equation and reference numbers conform to the letter.

### *A. Gaussian Belief Approximation for MM2*

We constrain the beliefs in the message passing scheme (6)–(8) to Gaussian pdfs. This is done by using the *information projection* approach [16], i.e., substituting for $q_k^{[t]}(\cdot)$ in (6)

$$\tilde{q}_k^{[t]}(\cdot) \triangleq \arg\min_{g \in \mathcal{G}} D\big[g \big\| q_k^{[t]}\big]. \tag{9}$$

Here, $D\big[g\|q\big] \triangleq \int g(\boldsymbol{x}) \ln \frac{g(\boldsymbol{x})}{q(\boldsymbol{x})} \mathrm{d}\boldsymbol{x}$ is the Kullback-Leibler divergence and $\mathcal{G}$ is the set of 4-D Gaussian pdfs $g(\boldsymbol{x}) = N(\boldsymbol{x}; \boldsymbol{\mu}, \boldsymbol{C})$ with covariance matrix of the form

$$\boldsymbol{C} = \begin{bmatrix} c_{\mathrm{p}} & c \\ c & c_{\mathrm{v}} \end{bmatrix} \otimes \mathbf{I}_2 .$$

We will denote the mean and covariance matrix of $\tilde{q}_k^{[t]}(\boldsymbol{x}_k^n) = N\big(\boldsymbol{x}_k^n; (\boldsymbol{\mu}_k^n)^{[t]}, (\boldsymbol{C}_k^n)^{[t]}\big)$ defined in (9) as

$$(\boldsymbol{\mu}_k^n)^{[t]} = \begin{bmatrix} (\boldsymbol{\mu}_{\mathrm{p},k}^n)^{[t]} \\ (\boldsymbol{\mu}_{\mathrm{v},k}^n)^{[t]} \end{bmatrix}, \qquad (\boldsymbol{C}_k^n)^{[t]} = \begin{bmatrix} (c_{\mathrm{p},k}^n)^{[t]} & (c_k^n)^{[t]} \\ (c_k^n)^{[t]} & (c_{\mathrm{v},k}^n)^{[t]} \end{bmatrix} \otimes \mathbf{I}_2 .$$

Because direct computation of the minimizer (9) is not feasible, we resort to an iterative method. To that end, we first derive an analytical expression of the objective function $D\big[g \big\| q_k^{[t]}\big]$ in (9), which we abbreviate by $F_k^{[t]}(\boldsymbol{\theta})$ with $\boldsymbol{\theta} \triangleq [\boldsymbol{\mu}^{\mathrm{T}} \; c_{\mathrm{p}} \; c_{\mathrm{v}} \; c]^{\mathrm{T}}$. Using the factorization in (6), this function can be expressed as

$$F_k^{[t]}(\boldsymbol{\theta}) = \int g(\boldsymbol{x}_k^n) \ln \frac{g(\boldsymbol{x}_k^n)}{\frac{1}{Z} m_{k\to k}(\boldsymbol{x}_k^n) \prod_{l \in \mathcal{N}_k^n} m_{l\to k}^{[t]}(\boldsymbol{p}_k^n)} \mathrm{d}\boldsymbol{x}_k^n$$

$$= \int g(\boldsymbol{x}_k^n) \ln \frac{g(\boldsymbol{x}_k^n)}{m_{k\to k}(\boldsymbol{x}_k^n)} \, \mathrm{d}\boldsymbol{x}_k^n - \int g(\boldsymbol{x}_k^n) \ln\Bigg( \prod_{l\in\mathcal{N}_k^n} m_{l\to k}^{[t]}(\boldsymbol{p}_k^n) \Bigg) \mathrm{d}\boldsymbol{x}_k^n + \ln Z$$

$$= D[g\| m_{k\to k}] - \sum_{l\in\mathcal{N}_k^n} G_{k,l}^{[t]}(\boldsymbol{\mu}_{\mathrm{p}}, c_{\mathrm{p}}) + \gamma, \tag{10}$$

where $\boldsymbol{\mu}_{\mathrm{p}}$ is the 2-D vector consisting of the first two entries of $\boldsymbol{\mu}$, $\gamma = \ln Z$ is a constant, and

$$G_{k,l}^{[t]}(\boldsymbol{\mu}_{\mathrm{p}}, c_{\mathrm{p}}) \triangleq \int N(\boldsymbol{x}_k^n; \boldsymbol{\mu}, \boldsymbol{C}) \ln m_{l\to k}^{[t]}(\boldsymbol{p}_k^n) \, \mathrm{d}\boldsymbol{x}_k^n$$
$$= \int N(\boldsymbol{p}_k^n; \boldsymbol{\mu}_{\mathrm{p}}, c_{\mathrm{p}}\mathbf{I}_2) \ln m_{l\to k}^{[t]}(\boldsymbol{p}_k^n) \, \mathrm{d}\boldsymbol{p}_k^n. \tag{11}$$

It remains to derive expressions of the terms $D[g\| m_{k\to k}]$ and $G_{k,l}^{[t]}(\boldsymbol{\mu}_{\mathrm{p}}, c_{\mathrm{p}})$ involved in (10). For an expression of $D[g\| m_{k\to k}]$, we note that for $k \in \mathcal{V}_{\mathrm{M}}^n \cap \mathcal{V}_{\mathrm{M}}^{n-1}$, due to the Gaussian $\tilde{q}_k^{[t]}(\boldsymbol{x}_k^n)$ and the linear-Gaussian model (1), the message in (7) (in which $q_k^{[t^*]}(\boldsymbol{x}_k^{n-1})$ is replaced by $\tilde{q}_k^{[t^*]}(\boldsymbol{x}_k^{n-1})$) is also Gaussian, i.e., $m_{k\to k}(\boldsymbol{x}_k^n) = N(\boldsymbol{x}_k^n; \boldsymbol{\eta}_k^n, \boldsymbol{\Sigma}_k^n)$. By using (1) and standard Gaussian integral identities [20], we obtain for $k \in \mathcal{V}_{\mathrm{M}}^n \cap \mathcal{V}_{\mathrm{M}}^{n-1}$

$$\boldsymbol{\eta}_k^n = \boldsymbol{F}(\boldsymbol{\mu}_k^{n-1})^{[t^*]}, \qquad \boldsymbol{\Sigma}_k^n = \boldsymbol{F}(\boldsymbol{C}_k^{n-1})^{[t^*]}\boldsymbol{F}^{\mathrm{T}} + \sigma_a^2 \boldsymbol{G}\boldsymbol{G}^{\mathrm{T}}. \tag{12}$$

For $k \in \mathcal{V}_{\mathrm{M}}^n \setminus \mathcal{V}_{\mathrm{M}}^{n-1}$, $\boldsymbol{\eta}_k^n$ and $\boldsymbol{\Sigma}_k^n$ equal, respectively, the mean and the covariance matrix of the Gaussian prior $p(\boldsymbol{x}_k^n) = N(\boldsymbol{x}_k^n; \boldsymbol{\eta}_k^n, \boldsymbol{\Sigma}_k^n)$. Accordingly, we obtain in either case [20]

$$D[g\| m_{k\to k}] = \frac{1}{2}\Big[\mathrm{tr}\big((\boldsymbol{\Sigma}_k^n)^{-1}\boldsymbol{C}\big) - \ln\det(\boldsymbol{C}) + (\boldsymbol{\mu}-\boldsymbol{\eta}_k^n)^{\mathrm{T}}(\boldsymbol{\Sigma}_k^n)^{-1}(\boldsymbol{\mu}-\boldsymbol{\eta}_k^n)\Big] + \gamma', \tag{13}$$

where $\gamma'$ is a constant.

To derive an analytic expression of $G_{k,l}^{[t]}(\boldsymbol{\mu}_{\mathrm{p}}, c_{\mathrm{p}})$, we first note that for $l \in \mathcal{V}_{\mathrm{M}}^n$, the pdf $q_l^{[t-1]}(\boldsymbol{x}_l^n)$ in (8) was replaced by the Gaussian pdf $\tilde{q}_l^{[t-1]}(\boldsymbol{x}_l^n)$. With a slight abuse of notation, we introduce the marginalized Gaussian pdf $\tilde{q}_l^{[t-1]}(\boldsymbol{p}_l^n) \triangleq \int \tilde{q}_l^{[t-1]}(\boldsymbol{x}_l^n) \mathrm{d}\boldsymbol{v}_l^n$. Note that for $l \in \mathcal{V}_{\mathrm{A}}^n$, the true position $\tilde{\boldsymbol{p}}_l^n$ is known. To obtain a unified notation, we introduce $\tilde{q}_l^{[t-1]}(\boldsymbol{p}_l^n) \triangleq \delta(\boldsymbol{p}_l^n - \tilde{\boldsymbol{p}}_l^n)$ for $l \in \mathcal{V}_{\mathrm{A}}^n$, i.e., $\tilde{q}_l^{[t-1]}(\boldsymbol{p}_l^n)$ is a Gaussian pdf with mean $\tilde{\boldsymbol{p}}_l^n$ and variance zero. The corresponding approximation of message $m_{l\to k}^{[t]}(\boldsymbol{p}_k^n)$ in (8) thus reads

$$\tilde{m}_{l\to k}^{[t]}(\boldsymbol{p}_k^n) = \exp\bigg( \int \tilde{q}_k^{[t-1]}(\boldsymbol{x}_l^n) \ln p(d_{k,l}^n | \boldsymbol{p}_k^n, \boldsymbol{p}_l^n) \, \mathrm{d}\boldsymbol{x}_l^n \bigg)$$
$$= \exp\bigg( \int \tilde{q}_k^{[t-1]}(\boldsymbol{p}_l^n) \ln p(d_{k,l}^n | \boldsymbol{p}_k^n, \boldsymbol{p}_l^n) \, \mathrm{d}\boldsymbol{p}_l^n \bigg).$$

By substituting $\tilde{m}_{l\to k}^{[t]}(\boldsymbol{p}_k^n)$ for $m_{l\to k}^{[t]}(\boldsymbol{p}_k^n)$ in (11), we obtain

$$G_{k,l}^{[t]}(\boldsymbol{\mu}_{\mathrm{p}}, c_{\mathrm{p}}) = \int N(\boldsymbol{p}_k^n; \boldsymbol{\mu}_{\mathrm{p}}, c_{\mathrm{p}}\mathbf{I}_2) \int \tilde{q}_l^{[t-1]}(\boldsymbol{p}_l^n) \ln p(d_{k,l}^n | \boldsymbol{p}_k^n, \boldsymbol{p}_l^n) \, \mathrm{d}\boldsymbol{p}_l^n \mathrm{d}\boldsymbol{p}_k^n$$
$$= \mathrm{E}_{p^{[t-1]}(\boldsymbol{p}_k^n, \boldsymbol{p}_l^n)}\big[\ln p(d_{k,l}^n | \boldsymbol{p}_k^n, \boldsymbol{p}_l^n)\big],$$

where $\mathrm{E}_{p^{[t-1]}(\boldsymbol{p}_k^n, \boldsymbol{p}_l^n)}[\cdot]$ denotes expectation with respect to the hypothetical pdf

$$p^{[t-1]}(\boldsymbol{p}_k^n, \boldsymbol{p}_l^n) \triangleq N(\boldsymbol{p}_k^n; \boldsymbol{\mu}_{\mathrm{p}}, c_{\mathrm{p}}\mathbf{I}_2) \, \tilde{q}_l^{[t-1]}(\boldsymbol{p}_l^n).$$

According to this hypothetical pdf, $\boldsymbol{p}_k^n$ and $\boldsymbol{p}_l^n$ are independent Gaussian random vectors.

Next, we introduce the auxiliary 2-D random vector

$$\boldsymbol{z}_{k,l}^n \triangleq \boldsymbol{p}_k^n - \boldsymbol{p}_l^n.$$

According to the hypothetical Gaussian pdf $p^{[t-1]}(\boldsymbol{p}_k^n, \boldsymbol{p}_l^n)$ of the random vector $\big[(\boldsymbol{p}_k^n)^{\mathrm{T}}\ (\boldsymbol{p}_l^n)^{\mathrm{T}}\big]^{\mathrm{T}}$, $\boldsymbol{z}_{k,l}^n$ is a Gaussian random vector with pdf $\tilde{p}^{[t-1]}(\boldsymbol{z}_{k,l}^n) = N(\boldsymbol{z}_{k,l}^n; \boldsymbol{\mu}_z, c_z\mathbf{I}_2)$, where $\boldsymbol{\mu}_z = \boldsymbol{\mu}_{\mathrm{p}} - (\boldsymbol{\mu}_{\mathrm{p},l}^n)^{[t-1]}$ and $c_z = c_{\mathrm{p}} + (c_{\mathrm{p},l}^n)^{[t-1]}$. For $l \in \mathcal{V}_{\mathrm{A}}^n$, in particular, $(\boldsymbol{\mu}_{\mathrm{p},l}^n)^{[t-1]} = \tilde{\boldsymbol{p}}_l^n$ and $(c_{\mathrm{p},l}^n)^{[t-1]} = 0$. Then, inserting for $p^{[t-1]}(\boldsymbol{p}_k^n, \boldsymbol{p}_l^n)$ and $p(d_{k,l}^n | \boldsymbol{p}_k^n, \boldsymbol{p}_l^n)$, it is straightforward to show that

$$\mathrm{E}_{p^{[t-1]}(\boldsymbol{p}_k^n, \boldsymbol{p}_l^n)}\big[\ln p(d_{k,l}^n | \boldsymbol{p}_k^n, \boldsymbol{p}_l^n)\big] = -\frac{1}{2\sigma_w^2}\,\mathrm{E}_{\tilde{p}^{[t-1]}(\boldsymbol{z}_{k,l}^n)}\big[(d_{k,l}^n - \|\boldsymbol{z}_{k,l}^n\|)^2\big] - \ln 2\pi\sigma_w^2,$$

where the expectation on the right hand side can be expanded as

$$\mathrm{E}_{\tilde{p}^{[t-1]}(\boldsymbol{z}_{k,l}^n)}\big[(d_{k,l}^n - \|\boldsymbol{z}_{k,l}^n\|)^2\big] = (d_{k,l}^n)^2 - 2d_{k,l}^n\,\mathrm{E}_{\tilde{p}^{[t-1]}(\boldsymbol{z}_{k,l}^n)}\big[\|\boldsymbol{z}_{k,l}^n\|\big] + \mathrm{E}_{\tilde{p}^{[t-1]}(\boldsymbol{z}_{k,l}^n)}\big[\|\boldsymbol{z}_{k,l}^n\|^2\big].$$

Because $\|z_{k,l}^n\|$ is a Rician random variable, we can express $\mathrm{E}_{\tilde{p}^{[t-1]}(\boldsymbol{z}_{k,l}^n)}\big[\|z_{k,l}^n\|\big]$ and $\mathrm{E}_{\tilde{p}^{[t-1]}(\boldsymbol{z}_{k,l}^n)}\big[\|z_{k,l}^n\|^2\big]$ by using the expressions of the first-order and second-order moments of a Rician random variable given in [21]. We finally obtain

$$G_{k,l}^{[t]}(\boldsymbol{\mu}_{\mathrm{p}}, c_{\mathrm{p}}) = -\frac{d_\mu^2 + 2c_{\mathrm{p}}}{2\sigma_w^2} + \frac{d_{k,l}^n}{\sigma_w^2}\sqrt{\frac{\pi C}{2}}\,M\!\left(-\frac{1}{2}; 1; -\frac{d_\mu^2}{2C}\right) + \gamma'', \tag{14}$$

where $d_\mu \triangleq \big\|\boldsymbol{\mu}_{\mathrm{p}} - (\boldsymbol{\mu}_{\mathrm{p},l}^n)^{[t-1]}\big\|$, $C \triangleq c_{\mathrm{p}} + (c_{\mathrm{p},l}^n)^{[t-1]}$, $M(\cdot\,;\cdot\,;\cdot)$ denotes the confluent hypergeometric function of the first kind [22], and $\gamma''$ is a constant.
